# Supplementary material for: Ultimate-rate quantum repeaters for quantum communications
Source: arXiv:2306.08816 source file (2023-06-15)
Supplement: Supplementary file 1 [file appendix_simple_repeater.tex]

%====================================================
%====================================================
%====================================================
%====================================================
%====================================================
%====================================================%====================================================%====================================================%====================================================%====================================================%====================================================%====================================================

%%==============
%%====================================================
\chapter{Some additional material about the simple repeater}\label{app:simple_repeater}
%%====================================================
